# Supplementary material for: Beyond Static Bias: Adaptive Multi-Fidelity Bandits with Improving Proxies
Source: arXiv:2605.08558 source file (2026-05-08)
Supplement: Supplementary file 1 [file appendix.tex]

\section{Additional Proof Details and Algorithmic Variants}
\label{app:proofs}

This appendix serves two purposes. First, it makes the current proof route for the RDFE benchmark more explicit by isolating the bookkeeping lemmas that connect phase-wise elimination to the oracle complexity $\mathsf{c}_k^\star(\varepsilon;\Lambda)$. Second, it records algorithmic variants that are useful for intuition and future extensions but are not the main algorithmic vehicle in the body of the paper.

\subsection{Proof strategy and bookkeeping}
\label{app:proof-strategy}

The main theorem is proved by combining three ingredients.

First, Lemma~\ref{lem:ci} gives a budget-uniform confidence event $\mathcal{E}_\Lambda$ on which both fidelities provide valid confidence intervals for the same target quantity $\mu_k^{(H)}$.

Second, once a phase is completed, every active arm has confidence radius at most $\varepsilon_r/8$. This implies a phase-end separation statement: if $\Delta_k\ge \varepsilon_r$, then arm $k$ cannot remain active after phase $r$.

Third, to upper bound the regret, we must relate the \emph{actual additional cost incurred during phase $r$} to the oracle cost complexity $\mathsf{c}_k^\star(\varepsilon_r;\Lambda)$. This is slightly more delicate than the proof sketch in the main text, because $\mathsf{c}_k^\star(\varepsilon_r;\Lambda)$ is defined as a \emph{from-scratch} certification cost, whereas the algorithm carries samples across phases. The remedy is a simple charging lemma: the additional phase-$r$ cost spent on arm $k$ is at most the corresponding oracle from-scratch cost at scale $\varepsilon_r$.

For bookkeeping, call a phase $r$ \emph{completed} if the algorithm finishes processing every arm in $\mathcal{S}_r$ and performs the elimination update that defines $\mathcal{S}_{r+1}$. Let $R_\Lambda$ denote the number of completed phases under budget $\Lambda$. For each arm $k$ and completed phase $r\le R_\Lambda$, let
\begin{equation}
\Delta \Lambda_{k,r}
\end{equation}
denote the additional cost spent on arm $k$ during phase $r$. If $k\notin \mathcal{S}_r$, we set $\Delta \Lambda_{k,r}:=0$.

\subsection{Proof of Lemma~\ref{lem:ci}}
\label{app:proof-lem-ci}

We prove that both the low-fidelity and high-fidelity confidence intervals cover the target mean $\mu_k^{(H)}$ uniformly over all arms and all sample counts up to the budget horizon.

For high fidelity, the claim is standard. By Assumption~\ref{ass:noise}, for each fixed arm $k$ and sample size $n$, the empirical mean of the first $n$ high-fidelity samples is $\sigma$-sub-Gaussian around $\mu_k^{(H)}$. By a uniform concentration bound over all $k\in[K]$ and all $1\le n\le T_\Lambda$, with probability at least $1-\delta/2$,
\begin{equation}
\left|
\hat{\mu}_{k,t}^{(H)}-\mu_k^{(H)}
\right|
\le
G_\Lambda\bigl(N_{k,t}^{(H)},\delta\bigr)
\end{equation}
for all arms $k$ and all rounds $t\le T_\Lambda$.

For low fidelity, recall the decomposition
\begin{equation}
\hat{\mu}_{k,t}^{(L)}-\mu_k^{(H)}
=
\bigl(
\hat{\mu}_{k,t}^{(L)}-\bar{\mu}_k^{(L)}(N_{k,t}^{(L)})
\bigr)
+
\bigl(
\bar{\mu}_k^{(L)}(N_{k,t}^{(L)})-\mu_k^{(H)}
\bigr).
\end{equation}
The first term is stochastic and is again controlled uniformly by a sub-Gaussian concentration bound: with probability at least $1-\delta/2$,
\begin{equation}
\left|
\hat{\mu}_{k,t}^{(L)}-\bar{\mu}_k^{(L)}(N_{k,t}^{(L)})
\right|
\le
G_\Lambda\bigl(N_{k,t}^{(L)},\delta\bigr)
\end{equation}
for all arms $k$ and all rounds $t\le T_\Lambda$.

For the second term, Assumption~\ref{ass:plugin} gives
\begin{equation}
\left|
\bar{\mu}_k^{(L)}(n)-\mu_k^{(H)}
\right|
\le
\frac{1}{n}\sum_{\tau=1}^{n}
\left|
\mu_k^{(L)}(\tau)-\mu_k^{(H)}
\right|
\le
\frac{U_k(n,\delta)}{n}
\le
B_k(n).
\end{equation}
Combining the stochastic and deterministic bounds yields
\begin{equation}
\left|
\hat{\mu}_{k,t}^{(L)}-\mu_k^{(H)}
\right|
\le
G_\Lambda\bigl(N_{k,t}^{(L)},\delta\bigr)
+
B_k\bigl(N_{k,t}^{(L)}\bigr),
\end{equation}
which is exactly the low-fidelity confidence interval. A union bound over the high-fidelity and low-fidelity events proves the claim.

\subsection{Auxiliary phase lemmas}
\label{app:aux-phase}

The next two lemmas isolate facts about completed phases that are used repeatedly in the proofs of Lemma~\ref{lem:elim} and Proposition~\ref{prop:cost}.

\begin{lemma}[Phase-end confidence width]
\label{lem:phase-width}
Suppose phase $r$ is completed and the event $\mathcal{E}_\Lambda$ in Lemma~\ref{lem:ci} holds. Then for every arm $k\in\mathcal{S}_r$,
\begin{equation}
\mu_k^{(H)}\in[\mathrm{LCB}_{k,r},\mathrm{UCB}_{k,r}]
\qquad\text{and}\qquad
\mathrm{UCB}_{k,r}-\mathrm{LCB}_{k,r}\le \varepsilon_r/4.
\end{equation}
\end{lemma}

\begin{proof}
Fix a completed phase $r$ and an arm $k\in\mathcal{S}_r$. By construction, phase $r$ queries arm $k$ until its relevant confidence radius is at most $\varepsilon_r/8$. If the chosen fidelity is low, then
\begin{equation}
G_\Lambda\bigl(N_k^{(L)},\delta\bigr)+B_k\bigl(N_k^{(L)}\bigr)\le \varepsilon_r/8,
\end{equation}
and hence
\begin{equation}
\mathrm{UCB}_{k,r}-\mathrm{LCB}_{k,r}
=
2\Bigl(
G_\Lambda\bigl(N_k^{(L)},\delta\bigr)+B_k\bigl(N_k^{(L)}\bigr)
\Bigr)
\le \varepsilon_r/4.
\end{equation}
If the chosen fidelity is high, then similarly
\begin{equation}
G_\Lambda\bigl(N_k^{(H)},\delta\bigr)\le \varepsilon_r/8,
\end{equation}
so
\begin{equation}
\mathrm{UCB}_{k,r}-\mathrm{LCB}_{k,r}
=
2G_\Lambda\bigl(N_k^{(H)},\delta\bigr)
\le \varepsilon_r/4.
\end{equation}
Coverage follows from Lemma~\ref{lem:ci}.
\end{proof}

\begin{lemma}[The optimal arm survives every completed phase]
\label{lem:opt-survives}
Suppose phase $r$ is completed and the event $\mathcal{E}_\Lambda$ holds. Then $k^\star\in\mathcal{S}_{r+1}$.
\end{lemma}

\begin{proof}
By Lemma~\ref{lem:phase-width},
\begin{equation}
\mathrm{UCB}_{k^\star,r}\ge \mu^\star
\qquad\text{and}\qquad
\mathrm{LCB}_{k^\star,r}\le \mu^\star.
\end{equation}
Since $\hat{k}_r$ is chosen to maximize $\mathrm{LCB}_{k,r}$ over $k\in\mathcal{S}_r$,
\begin{equation}
\mathrm{LCB}_{\hat{k}_r,r}\ge \mathrm{LCB}_{k^\star,r}.
\end{equation}
Therefore
\begin{equation}
\mathrm{UCB}_{k^\star,r}
\ge
\mathrm{LCB}_{k^\star,r}
\ge
\mathrm{LCB}_{\hat{k}_r,r}-\varepsilon_r/4,
\end{equation}
so $k^\star$ is not eliminated by the phase-$r$ elimination rule.
\end{proof}

\subsection{Proof of Lemma~\ref{lem:elim}}
\label{app:proof-lem-elim}

We now prove the phase-elimination statement using the actual elimination threshold in Algorithm~\ref{alg:rdfe}.

Assume phase $r$ is completed and the event $\mathcal{E}_\Lambda$ holds. By Lemma~\ref{lem:phase-width}, for every arm $k\in\mathcal{S}_r$,
\begin{equation}
\mathrm{UCB}_{k,r}\le \mu_k^{(H)}+\varepsilon_r/8.
\end{equation}
Also, by Lemma~\ref{lem:opt-survives},
\begin{equation}
\mathrm{LCB}_{\hat{k}_r,r}\ge \mathrm{LCB}_{k^\star,r}\ge \mu^\star-\varepsilon_r/8.
\end{equation}
Hence
\begin{equation}
\mathrm{LCB}_{\hat{k}_r,r}-\varepsilon_r/4
\ge
\mu^\star-\frac{3\varepsilon_r}{8}.
\end{equation}

If $\Delta_k=\mu^\star-\mu_k^{(H)}\ge \varepsilon_r$, then
\begin{equation}
\mathrm{UCB}_{k,r}
\le
\mu_k^{(H)}+\varepsilon_r/8
=
\mu^\star-\Delta_k+\varepsilon_r/8
\le
\mu^\star-\frac{7\varepsilon_r}{8}
<
\mu^\star-\frac{3\varepsilon_r}{8}
\le
\mathrm{LCB}_{\hat{k}_r,r}-\varepsilon_r/4.
\end{equation}
Therefore arm $k$ fails the phase-$r$ survival test and is eliminated by the end of phase $r$.

\subsection{A single-phase cost lemma}
\label{app:phase-cost}

The next lemma is the key bookkeeping step missing from the shorter proof sketch in the main text. It upper bounds the \emph{actual additional cost} incurred during a completed phase by the oracle certification cost at that phase resolution.

\begin{lemma}[Single-phase additional cost upper bound]
\label{lem:phase-cost}
Fix a completed phase $r\le R_\Lambda$ and an arm $k\in\mathcal{S}_r$. Then
\begin{equation}
\Delta\Lambda_{k,r}
\le
\mathsf{c}_k^\star(\varepsilon_r;\Lambda).
\end{equation}
\end{lemma}

\begin{proof}
Let
\begin{equation}
n_{k,L}(\varepsilon_r)
:=
\min\Bigl\{
n\ge 1:
G_\Lambda(n,\delta)+B_k(n)\le \varepsilon_r/8
\Bigr\},
\end{equation}
and
\begin{equation}
n_H(\varepsilon_r)
:=
\min\Bigl\{
n\ge 1:
G_\Lambda(n,\delta)\le \varepsilon_r/8
\Bigr\}.
\end{equation}
Then
\begin{equation}
\mathsf{c}_k^{(L)}(\varepsilon_r;\Lambda)
=
\lambda^{(L)} n_{k,L}(\varepsilon_r),
\qquad
\mathsf{c}^{(H)}(\varepsilon_r;\Lambda)
=
\lambda^{(H)} n_H(\varepsilon_r).
\end{equation}

If phase $r$ selects low fidelity for arm $k$, then the algorithm continues querying low fidelity until
\begin{equation}
G_\Lambda\bigl(N_k^{(L)},\delta\bigr)+B_k\bigl(N_k^{(L)}\bigr)\le \varepsilon_r/8.
\end{equation}
Therefore the number of \emph{additional} low-fidelity pulls made during phase $r$ is at most
\begin{equation}
\bigl(n_{k,L}(\varepsilon_r)-N_{k,r-1}^{(L)}\bigr)_+,
\end{equation}
and hence
\begin{equation}
\Delta\Lambda_{k,r}
\le
\lambda^{(L)}
\bigl(n_{k,L}(\varepsilon_r)-N_{k,r-1}^{(L)}\bigr)_+
\le
\lambda^{(L)}n_{k,L}(\varepsilon_r)
=
\mathsf{c}_k^{(L)}(\varepsilon_r;\Lambda).
\end{equation}

If phase $r$ selects high fidelity for arm $k$, the same reasoning gives
\begin{equation}
\Delta\Lambda_{k,r}
\le
\lambda^{(H)}
\bigl(n_H(\varepsilon_r)-N_{k,r-1}^{(H)}\bigr)_+
\le
\lambda^{(H)}n_H(\varepsilon_r)
=
\mathsf{c}^{(H)}(\varepsilon_r;\Lambda).
\end{equation}

Since phase $r$ chooses
\begin{equation}
m_{k,r}\in \arg\min\bigl\{\mathsf{c}_k^{(L)}(\varepsilon_r;\Lambda),\mathsf{c}^{(H)}(\varepsilon_r;\Lambda)\bigr\},
\end{equation}
we conclude in either case that
\begin{equation}
\Delta\Lambda_{k,r}
\le
\mathsf{c}_k^\star(\varepsilon_r;\Lambda).
\end{equation}
\end{proof}

\subsection{Proof of Proposition~\ref{prop:cost}}
\label{app:proof-prop-cost}

Fix a suboptimal arm $k\neq k^\star$ and define
\begin{equation}
r_k:=\min\{r:\varepsilon_r\le \Delta_k/2\}.
\end{equation}
By Lemma~\ref{lem:elim}, if phase $r$ is completed and $r\ge r_k$, then arm $k$ is eliminated by the end of phase $r$. Therefore arm $k$ can only incur phase-based exploration cost while active in phases $1,\dots,r_k$.

More precisely, the total additional exploration cost incurred on arm $k$ before elimination is bounded by
\begin{equation}
\sum_{r\le \min\{r_k,R_\Lambda\}} \Delta\Lambda_{k,r}
\le
\sum_{r\le r_k}\Delta\Lambda_{k,r}.
\end{equation}
Applying Lemma~\ref{lem:phase-cost} phase by phase gives
\begin{equation}
\sum_{r\le r_k}\Delta\Lambda_{k,r}
\le
\sum_{r\le r_k}\mathsf{c}_k^\star(\varepsilon_r;\Lambda).
\end{equation}
Now invoke Assumption~\ref{ass:dyadic} to obtain
\begin{equation}
\sum_{r\le r_k}\mathsf{c}_k^\star(\varepsilon_r;\Lambda)
\le
C_{\mathrm{dyad}}\,
\mathsf{c}_k^\star(\varepsilon_{r_k};\Lambda).
\end{equation}
Finally, by definition of $r_k$,
\begin{equation}
\varepsilon_{r_k}\le \Delta_k/2
\qquad\text{and}\qquad
\varepsilon_{r_k-1}>\Delta_k/2,
\end{equation}
so
\begin{equation}
\Delta_k/4<\varepsilon_{r_k}\le \Delta_k/2.
\end{equation}
Since $\mathsf{c}_k^\star(\varepsilon;\Lambda)$ is nonincreasing in $\varepsilon$ by definition,
\begin{equation}
\mathsf{c}_k^\star(\varepsilon_{r_k};\Lambda)
\le
\mathsf{c}_k^\star(\Delta_k/4;\Lambda).
\end{equation}
Combining the displays yields
\begin{equation}
\sum_{r\le r_k}\Delta\Lambda_{k,r}
\le
C\,\mathsf{c}_k^\star(\Delta_k/4;\Lambda)
\end{equation}
for some absolute constant $C>0$, which proves the proposition.

\subsection{Proof of Theorem~\ref{thm:main}}
\label{app:proof-thm-main}

Work on the event $\mathcal{E}_\Lambda$, which holds with probability at least $1-\delta$ by Lemma~\ref{lem:ci}. Fix a suboptimal arm $k\neq k^\star$. Every unit of cost spent on arm $k$ contributes at most $\Delta_k$ to the cost-weighted pseudo-regret, so the regret from arm $k$ is bounded by
\begin{equation}
R_k
\le
\Delta_k
\left(
\text{total cost spent on arm $k$ before elimination}
\right).
\end{equation}

The phase-based exploration cost incurred on arm $k$ before elimination is controlled by Proposition~\ref{prop:cost}, which gives
\begin{equation}
R_k
\le
C\,\Delta_k\,\mathsf{c}_k^\star(\Delta_k/4;\Lambda).
\end{equation}
Summing over all suboptimal arms yields the main term
\begin{equation}
\sum_{k\neq k^\star}
C\,\Delta_k\,\mathsf{c}_k^\star(\Delta_k/4;\Lambda).
\end{equation}

The warm-start contributes one low-fidelity query and one high-fidelity query per arm. Under the standard normalization $\mu_k^{(H)}\in[0,1]$, one has $\Delta_k\le 1$, so the warm-start contribution is at most
\begin{equation}
O\bigl(K(\lambda^{(L)}+\lambda^{(H)})\bigr).
\end{equation}
If one prefers not to use this normalization, the same step yields the slightly more explicit term
\begin{equation}
\sum_{k\neq k^\star}\Delta_k\bigl(\lambda^{(L)}+\lambda^{(H)}\bigr),
\end{equation}
which can be carried throughout unchanged.

Finally, the theorem statement allows an additional explicit lower-order slack term
\begin{equation}
C_3\lambda^{(H)}\log\!\left(\frac{4KT_\Lambda^2}{\delta}\right),
\end{equation}
which can be retained to absorb uniform-confidence calibration constants and other negligible bookkeeping terms without affecting the benchmark interpretation. Combining the displays proves Theorem~\ref{thm:main}.

\subsection{Proof of Corollary~\ref{cor:gap}}
\label{app:proof-cor-gap}

Fix $\varepsilon\in(0,1]$ and partition the suboptimal arms into
\begin{equation}
\mathcal{A}_\varepsilon := \{k\neq k^\star:\Delta_k\ge \varepsilon\},
\qquad
\mathcal{B}_\varepsilon := \{k\neq k^\star:\Delta_k<\varepsilon\}.
\end{equation}
For the first set,
\begin{equation}
\sum_{k\in\mathcal{A}_\varepsilon}
\Delta_k\,\mathsf{c}_k^\star(\Delta_k/4;\Lambda)
\le
K\sup_{x\ge \varepsilon} x\,\mathsf{c}^\star(x;\Lambda).
\end{equation}
For the second set, each selected arm contributes at most $\varepsilon$ regret per unit cost, so the total contribution is at most $\Lambda\varepsilon$. Applying Theorem~\ref{thm:main} and optimizing over $\varepsilon$ yields the claim.

\subsection{A plug-in polynomial-envelope specialization}
\label{app:poly}

Suppose the cumulative mismatch certificate satisfies
\begin{equation}
U_k(n,\delta)\le \Gamma_k n^{1-\alpha}
\qquad\text{for some } \alpha>0.
\end{equation}
Then the selected-average envelope obeys
\begin{equation}
B_k(n)
=
\sup_{s\ge n}\frac{U_k(s,\delta)}{s}
\le
\Gamma_k n^{-\alpha}.
\end{equation}
Accordingly, the low-fidelity confidence radius takes the form
\begin{equation}
G_\Lambda(n,\delta)+B_k(n)
\lesssim
\sqrt{\frac{\log T_\Lambda}{n}}+\Gamma_k n^{-\alpha}.
\end{equation}
Consequently,
\begin{equation}
\mathsf{c}_k^{(L)}(\varepsilon;\Lambda)
\lesssim
\lambda^{(L)}
\max\left\{
\frac{\log T_\Lambda}{\varepsilon^2},
\left(\frac{\Gamma_k}{\varepsilon}\right)^{1/\alpha}
\right\}.
\end{equation}
This makes the trade-off explicit: low fidelity is attractive when its bias certificate decays quickly relative to its lower query cost, while high fidelity becomes preferable once the target resolution becomes sufficiently fine.

\subsection{Appendix-only threshold-based adaptive continuation companion}
\label{app:threshold-companion}

For completeness, we record the earlier threshold/continuation-style two-fidelity policy that originally motivated the current oracle benchmark. This procedure is no longer the headline algorithm of the paper, but it remains useful as an online, myopic counterpart to the phase-based RDFE rule.

Define the appendix-only effective low-fidelity gap by
\begin{equation}
\widetilde{\Delta}_k^{(L)}(n)
:=
\mu^\star-\bar{\mu}_k^{(L)}(n)-B_k(n),
\qquad
k\neq k^\star.
\end{equation}
For an additional block of $s$ low-fidelity queries from selected count $n$, define
\begin{equation}
\widetilde{V}_k(n,s)
:=
B_k(n)-B_k(n+s),
\qquad s\ge 1.
\end{equation}

At each round, the appendix-only threshold rule aggregates the two fidelity-specific confidence bounds through
\begin{equation}
\mathrm{UCB}_{k,t}
:=
\min_{m\in\{L,H\}}\mathrm{UCB}_{k,t}^{(m)},
\qquad
\mathrm{LCB}_{k,t}
:=
\max_{m\in\{L,H\}}\mathrm{LCB}_{k,t}^{(m)},
\end{equation}
selects
\begin{equation}
I_t\in\arg\max_{k\in[K]}\mathrm{UCB}_{k,t},
\end{equation}
and then uses a local continuation test based on the envelope shrinkage
\begin{equation}
\widetilde{V}_{k,t}(s)
:=
\widetilde{V}_k\!\left(N_{k,t}^{(L)},s\right)
=
B_k\!\left(N_{k,t}^{(L)}\right)-B_k\!\left(N_{k,t}^{(L)}+s\right).
\end{equation}
Specifically, it keeps querying low fidelity while the statistical radius remains above a threshold $\gamma$, and after crossing that threshold allows at most $S_0$ additional low-fidelity pulls if
\begin{equation}
\widetilde{V}_{I_t,t}(s)\ge 2\eta\gamma
\end{equation}
for some admissible look-ahead length $s$.

\begin{algorithm}[t]
\caption{Threshold-Based Adaptive Continuation Companion}
\label{alg:threshold-companion}
\begin{algorithmic}[1]
\Require budget $\Lambda$, arm set $[K]$, costs $\lambda^{(L)},\lambda^{(H)}$, threshold $\gamma$, ratio $\eta$, continuation cap $S_0$
\State query each arm once at low fidelity and once at high fidelity
\State initialize all empirical means, counts, and continuation counters
\While{cumulative cost $\le \Lambda$}
    \State construct $\mathrm{UCB}_{k,t}^{(L)},\mathrm{LCB}_{k,t}^{(L)},\mathrm{UCB}_{k,t}^{(H)},\mathrm{LCB}_{k,t}^{(H)}$ for all $k\in[K]$
    \State compute $\mathrm{UCB}_{k,t}=\min_{m\in\{L,H\}}\mathrm{UCB}_{k,t}^{(m)}$
    \State select $I_t\in\arg\max_{k\in[K]}\mathrm{UCB}_{k,t}$
    \If{$G_\Lambda(N_{I_t,t}^{(L)},\delta)\ge \gamma$}
        \State set $m_t=L$
    \ElsIf{$A_{I_t,t}<S_0$ and $\widetilde{V}_{I_t,t}(s)\ge 2\eta\gamma$ for some $1\le s\le S_0-A_{I_t,t}$}
        \State set $m_t=L$ and update $A_{I_t,t}\leftarrow A_{I_t,t}+1$
    \Else
        \State set $m_t=H$
    \EndIf
    \State query arm $I_t$ at fidelity $m_t$ and update empirical means and counts
\EndWhile
\end{algorithmic}
\end{algorithm}

The point of recording this algorithm is not to reposition the paper around it. Rather, it provides intuition for how a round-by-round rule can try to mimic the benchmark logic of RDFE using only local continuation tests. Its analysis typically relies on additional monotonicity and continuation-gain assumptions, and its theorem statements are more naturally case-based. For the present paper, the oracle phase-elimination route remains the cleanest submission-level vehicle.

\subsection{A dynamic-good-fidelity LUCB variant for multi-fidelity bandits}
\label{app:dgf-lucb}

We now describe a more general online LUCB-style certification primitive for the multi-fidelity setting. Let the fidelity set be
\begin{equation}
\mathcal{M}:=\{1,\dots,M\},
\end{equation}
where fidelity $M$ is the target fidelity and lower fidelities may evolve with their selected counts.

For each arm $k$ and fidelity $m\in\mathcal{M}$, let $N_{k,t}^{(m)}$ be the number of queries of arm $k$ at fidelity $m$ up to round $t$, and let $\hat{\mu}_{k,t}^{(m)}$ denote the corresponding empirical mean. Assume that each non-target fidelity $m<M$ is equipped with a plug-in cumulative mismatch certificate $U_k^{(m)}(\cdot,\delta)$, and define
\begin{equation}
B_k^{(m)}(n)
:=
\sup_{s\ge n}\frac{U_k^{(m)}(s,\delta)}{s},
\qquad m<M,
\end{equation}
while $B_k^{(M)}(n)\equiv 0$.

For each arm $k$, round $t$, and fidelity $m\in\mathcal{M}$, define
\begin{equation}
\operatorname{rad}_{k,t}^{(m)}
:=
G_\Lambda\bigl(N_{k,t}^{(m)},\delta\bigr)+B_k^{(m)}\bigl(N_{k,t}^{(m)}\bigr),
\end{equation}
and
\begin{equation}
\mathrm{UCB}_{k,t}^{(m)}
:=
\hat{\mu}_{k,t}^{(m)}+\operatorname{rad}_{k,t}^{(m)},
\qquad
\mathrm{LCB}_{k,t}^{(m)}
:=
\hat{\mu}_{k,t}^{(m)}-\operatorname{rad}_{k,t}^{(m)}.
\end{equation}
The aggregated arm-level bounds are
\begin{equation}
\mathrm{UCB}_{k,t}
:=
\min_{m\in\mathcal{M}} \mathrm{UCB}_{k,t}^{(m)},
\qquad
\mathrm{LCB}_{k,t}
:=
\max_{m\in\mathcal{M}} \mathrm{LCB}_{k,t}^{(m)}.
\end{equation}

At round $t$, let
\begin{equation}
\ell_t \in \operatorname*{arg\,max}_{k\in[K]} \mathrm{UCB}_{k,t},
\qquad
u_t \in \operatorname*{arg\,max}_{k\in[K]\setminus\{\ell_t\}} \mathrm{UCB}_{k,t}
\end{equation}
denote the empirical best arm and runner-up, respectively, and define the current critical scale by
\begin{equation}
\varepsilon_t := \mathrm{UCB}_{\ell_t,t}-\mathrm{LCB}_{u_t,t}.
\end{equation}

For a target resolution $\varepsilon>0$, define the remaining certification cost of arm $k$ at fidelity $m\in\mathcal{M}$ by
\begin{equation}
\mathsf{c}_{k,t}^{(m)}(\varepsilon)
:=
\lambda^{(m)}
\Bigl(
\min
\bigl\{
n \ge N_{k,t}^{(m)} :
G_\Lambda(n,\delta)+B_k^{(m)}(n)\le \varepsilon/8
\bigr\}
-
N_{k,t}^{(m)}
\Bigr)_+.
\end{equation}
The online fidelity rule then chooses, for each critical arm $k\in\{\ell_t,u_t\}$,
\begin{equation}
m_{k,t}
\in
\operatorname*{arg\,min}_{m\in\mathcal{M}}
\mathsf{c}_{k,t}^{(m)}(\varepsilon_t).
\end{equation}

\begin{algorithm}[t]
\caption{Multi-Fidelity Dynamic-Good-Fidelity LUCB (MF-DGF-LUCB)}
\label{alg:mf-dgf-lucb}
\begin{algorithmic}[1]
\Require confidence level $\delta$, budget $\Lambda$
\State initialize all counts $N_{k,0}^{(m)}\gets 0$ and empirical means $\hat{\mu}_{k,0}^{(m)}\gets 0$
\For{$t=1,2,\dots$ while cumulative cost $\le \Lambda$}
    \For{each arm $k\in[K]$ and fidelity $m\in\mathcal{M}$}
        \State compute
        \[
        \mathrm{UCB}_{k,t}^{(m)}
        =
        \hat{\mu}_{k,t}^{(m)}
        +
        G_\Lambda\bigl(N_{k,t}^{(m)},\delta\bigr)
        +
        B_k^{(m)}\bigl(N_{k,t}^{(m)}\bigr),
        \]
        \[
        \mathrm{LCB}_{k,t}^{(m)}
        =
        \hat{\mu}_{k,t}^{(m)}
        -
        G_\Lambda\bigl(N_{k,t}^{(m)},\delta\bigr)
        -
        B_k^{(m)}\bigl(N_{k,t}^{(m)}\bigr)
        \]
    \EndFor
    \For{each arm $k\in[K]$}
        \State aggregate
        \[
        \mathrm{UCB}_{k,t} := \min_{m\in\mathcal{M}} \mathrm{UCB}_{k,t}^{(m)},
        \qquad
        \mathrm{LCB}_{k,t} := \max_{m\in\mathcal{M}} \mathrm{LCB}_{k,t}^{(m)}
        \]
    \EndFor
    \State choose
    \[
    \ell_t \in \operatorname*{arg\,max}_{k\in[K]} \mathrm{UCB}_{k,t},
    \qquad
    u_t \in \operatorname*{arg\,max}_{k\in[K]\setminus\{\ell_t\}} \mathrm{UCB}_{k,t}
    \]
    \If{$\mathrm{LCB}_{\ell_t,t} > \mathrm{UCB}_{u_t,t}$}
        \State \Return $\ell_t$
    \EndIf
    \State set
    \[
    \varepsilon_t \gets \mathrm{UCB}_{\ell_t,t} - \mathrm{LCB}_{u_t,t}
    \]
    \For{each critical arm $k\in\{\ell_t,u_t\}$}
        \State choose
        \[
        m_{k,t}
        \in
        \operatorname*{arg\,min}_{m\in\mathcal{M}}
        \mathsf{c}_{k,t}^{(m)}(\varepsilon_t)
        \]
        \State query arm $k$ at fidelity $m_{k,t}$ and update $N_{k,t}^{(m_{k,t})}$ and $\hat{\mu}_{k,t}^{(m_{k,t})}$
    \EndFor
\EndFor
\State \Return the empirically best arm according to the final aggregated confidence bounds
\end{algorithmic}
\end{algorithm}

This algorithm is genuinely multi-fidelity: it chooses among all fidelities in $\mathcal{M}$ at each round. The preferred fidelity is not fixed in advance; it is chosen relative to the current critical scale $\varepsilon_t$ through the family of remaining certification costs
\begin{equation}
\bigl\{
\mathsf{c}_{k,t}^{(m)}(\varepsilon_t)
\bigr\}_{m\in\mathcal{M}}.
\end{equation}

\begin{proposition}[Certification-cost comparison; proof sketch only]
\label{prop:mf-dgf-shadow}
Fix a budget $\Lambda>0$ and suppose that an analogous multi-fidelity confidence event $\mathcal{E}_\Lambda^{\mathrm{MF}}$ holds for the aggregated confidence bounds. Assume further that:
\begin{enumerate}
    \item Assumption~\ref{ass:dyadic} holds;
    \item the critical-scale process $(\varepsilon_t)_t$ is nonincreasing up to a universal constant factor between successive certification stages;
    \item for every critical arm $k\in\{\ell_t,u_t\}$, the chosen fidelity minimizes the remaining certification cost at scale $\varepsilon_t$ up to a universal constant factor.
\end{enumerate}
Then every suboptimal arm $k\neq k^\star$ incurs total certification cost
\begin{equation}
O\left(
\sum_{r\le r_k}\mathsf{c}_k^\star(\varepsilon_r;\Lambda)
\right)
=
O\left(
\mathsf{c}_k^\star(\Delta_k/4;\Lambda)
\right),
\qquad
r_k:=\min\{r:\varepsilon_r\le \Delta_k/2\},
\end{equation}
where
\begin{equation}
\mathsf{c}_k^\star(\varepsilon;\Lambda)
:=
\min_{m\in\mathcal{M}} \mathsf{c}_k^{(m)}(\varepsilon;\Lambda).
\end{equation}
Consequently, if Algorithm~\ref{alg:mf-dgf-lucb} is used as the certification primitive inside an elimination wrapper, the resulting procedure satisfies a regret bound of the same qualitative form as Theorem~\ref{thm:main}.
\end{proposition}

\begin{proof}[Proof roadmap]
The argument has four steps.

\paragraph{Step 1: validity of aggregated confidence bounds.}
On the good event $\mathcal{E}_\Lambda^{\mathrm{MF}}$, for every arm $k$ and every round $t$, the aggregated confidence interval
\begin{equation}
[\mathrm{LCB}_{k,t},\,\mathrm{UCB}_{k,t}]
\end{equation}
contains the target mean $\mu_k^{(M)}$.

\paragraph{Step 2: critical-arm separation once the current scale is sufficiently small.}
One first relates the widths of the current critical arms $\ell_t$ and $u_t$ to the online critical scale
\begin{equation}
\varepsilon_t := \mathrm{UCB}_{\ell_t,t}-\mathrm{LCB}_{u_t,t}.
\end{equation}
Once this relation is established, the same confidence-separation argument as in Lemma~\ref{lem:elim} shows that any suboptimal arm $k$ with $\Delta_k \ge c\,\varepsilon_t$ can no longer remain critical, for a suitable absolute constant $c>0$.

\paragraph{Step 3: coupling to a shadow dyadic process.}
One then compares the online critical-scale process $(\varepsilon_t)_t$ with a dyadic grid
\begin{equation}
\varepsilon_r := 2^{-r},
\qquad r=1,2,\dots.
\end{equation}
The objective is to show that the online process does not revisit substantially finer scales too many times before the certification work required at a coarser scale has been completed. Formally, one needs a per-band charging lemma asserting that for each suboptimal arm $k$ and each dyadic band corresponding to $\varepsilon_r$, the total cost spent on querying arm $k$ while the online critical scale remains in that band is bounded by
\begin{equation}
O\bigl(\mathsf{c}_k^\star(\varepsilon_r;\Lambda)\bigr).
\end{equation}

\paragraph{Step 4: summation over dyadic scales.}
Once the per-band charging statement is established, the total certification cost charged to a suboptimal arm $k$ is bounded by
\begin{equation}
O\left(
\sum_{r\le r_k}\mathsf{c}_k^\star(\varepsilon_r;\Lambda)
\right),
\qquad
r_k := \min\{r:\varepsilon_r\le \Delta_k/2\}.
\end{equation}
Assumption~\ref{ass:dyadic} then yields
\begin{equation}
\sum_{r\le r_k}\mathsf{c}_k^\star(\varepsilon_r;\Lambda)
=
O\left(\mathsf{c}_k^\star(\Delta_k/4;\Lambda)\right).
\end{equation}
Embedding this certification primitive into an elimination wrapper recovers the stated theorem shape.
\end{proof}
