# Supplementary material for: Beyond Static Bias: Adaptive Multi-Fidelity Bandits with Improving Proxies
Source: arXiv:2605.08558 source file (2026-05-08)
Supplement: Supplementary file 2 [file llm_final_main_metrics.tex]

\begin{table}[t]
\centering
\caption{
Controlled LLM-policy experiment at final budget $\Lambda=256000$.
We report target simple regret, computed as the cost-weighted terminal regret divided by $\Lambda$, together with best-policy identification accuracy.
Lower regret is better.
}
\label{tab:llm-main-metrics}
\small
\begin{tabular}{lccc}
\toprule
Algorithm & Target simple regret & Best-policy acc. & High calls \\
\midrule
TACC & \textbf{0.0120 $\pm$ 0.0009} & 0.400 & 510.0 \\
High-only UCB & 0.0212 $\pm$ 0.0001 & 0.325 & 512.0 \\
Static MF-UCB & 0.0137 $\pm$ 0.0010 & 0.342 & 510.0 \\
Dynamic no-cont. & 0.0149 $\pm$ 0.0013 & 0.383 & 511.0 \\
Weak-only fixed & 0.0229 $\pm$ 0.0001 & 0.025 & 0.0 \\
\bottomrule
\end{tabular}
\end{table}
